# Supplementary material for: A three-axis Nanopositioner based on Near-Field Acoustic Levitation and Electromagnetic Actuation
Source: arXiv:2503.19175 source file (2025-04-23)
Supplement: Supplementary file 1 [file Supplementary.pdf]

# Supplementary Information

K. S. Vikrant, Prosanto Biswas, and S. O. Reza Moheimani, Fellow, IEEE

## Supplementary Note 1: Relationship Between the Stiffness Along the X-, Y-, and Z-Axes

Let $\mathbf{B} = [B_x\, B_y\, B_z]^T$ represent the resultant magnetic field generated by all four zones of the electromagnetic coil. Then, the stiffness components along the X-, Y-, and Z-axes for the magnetic plate made of $4n$ magnets, where $n$ represents the number of magnets in each zone, are given by:

$$k_x = -\frac{\partial F_x}{\partial x} = -2nM \int_V \partial_{xx} B_z \, dV, \tag{1}$$

$$k_y = -\frac{\partial F_y}{\partial y} = -2nM \int_V \partial_{yy} B_z \, dV, \tag{2}$$

$$k_z = -\frac{\partial F_a}{\partial z} - \frac{\partial F_z}{\partial z} = k_a - 2nM \int_V \partial_{zz} B_z \, dV, \tag{3}$$

where $k_a$ represents the acoustic stiffness and is defined as $k_a = -\frac{\partial F_a}{\partial z}$. Thus, the total stiffness becomes:

$$k_x + k_y + k_z = k_a - 2nM \int_V \nabla^2 B_z \, dV. \tag{4}$$

Since $\nabla \cdot \mathbf{B} = 0$, it follows that $\partial_z(\nabla \cdot \mathbf{B}) = 0$, or equivalently:

$$\partial_{zx} B_x + \partial_{zy} B_y + \partial_{zz} B_z = \partial_x(\partial_z B_x) + \partial_y(\partial_z B_y) + \partial_{zz} B_z = 0. \tag{5}$$

Given that $\nabla \times \mathbf{B} = 0$, we can assume $\partial_z B_x = \partial_x B_z$ and $\partial_z B_y = \partial_y B_z$. Substituting into Equation (5), we obtain:

$$\partial_{xx} B_z + \partial_{yy} B_z + \partial_{zz} B_z = \nabla^2 B_z = 0. \tag{6}$$

Substituting Equation (6) into Equation (4), we find:

$$k_x + k_y + k_z = k_a. \tag{7}$$

This fundamental relationship is valid for any hybrid positioner based on self-stabilizing levitation (e.g., diamagnetic, acoustic) and electromagnetic actuation [1]. It reveals that the total stiffness along the X-, Y-, and Z-axes is equal to the stiffness provided by the self-stable

levitation technique, in this case, the acoustic stiffness, $k_a$. Since the acoustic stiffness $k_a$ generated in the NFAL technique is multiple orders of magnitude higher than the stiffness generated by other self-stabilization-based levitation techniques, the hybrid positioner based on NFAL provides higher positioning bandwidth along all three axes. For the NFAL-based positioner reported in the main manuscript, the acoustic stiffness is approximately $5\,\mathrm{kN/m}$, which is three orders of magnitude larger than the diamagnetic stiffness previously reported in [1, 2].

# Supplementary Note 2: Effect of Finite Track Dimensions on the Electromagnetic Field

In this section, we compare the magnetic field $B_z$ generated by the idealized electromagnetic coil described in the modeling section with the field produced by the actual fabricated coil used in the experiments. The analytical model presented in Section III of the main manuscript assumes that each current-carrying track consists of an infinite number of infinitely long, infinitesimally thin parallel conductors spaced at intervals of $p/2$. In contrast, the fabricated track contains only 22 parallel copper conductors, each with a finite length of $74\,\mathrm{mm}$, a width of $127\,\mu\mathrm{m}$, and a thickness of $35\,\mu\mathrm{m}$. As a result, the actual magnetic field $B_z$ deviates slightly from the idealized model, particularly near the coil boundaries.

We computed the magnetic field $B_z$ generated by one of the fabricated tracks using Finite Element Analysis (FEA), and compared the result with the analytical expression. Specifically, the Ansys Maxwell module was used to simulate the magnetic field generated by the track $I_{1x}$. Figure 1(a) illustrates the geometry used in the FEA model. Figure 1(b) shows the computed distribution of $B_z$ in the XZ-plane at $y = 0$, for a current of $I_{1x} = 0.4\,\mathrm{A}$. The magnetic field $B_z$ exhibits periodic variation along the X-axis with a fundamental period $p$, and its magnitude decreases with increasing Z-position. The plotted Z-range from $z = 800\,\mu\mathrm{m}$ to $z = 1300\,\mu\mathrm{m}$ corresponds to the lower and upper surfaces of the magnetic plate, respectively.

To characterize the periodic behavior along the X-direction, the magnetic field $B_z$ was extracted across the coil width at a fixed height of $z = 1050\,\mu\mathrm{m}$ (indicated by the horizontal dotted line in Fig. 1(b)). The FEA-computed magnetic field is plotted in red in Fig. 1(c), while the ideal field predicted by Equation 3 of the main manuscript is shown as a black dotted line. The results show that the computed field closely follows a sinusoidal pattern and matches the modeled field away from coil edges, with minor deviations near boundaries due to edge effects.

Additionally, Fig. 1(d) presents the variation of $B_z$ with Z at $x = 0\,\mu\mathrm{m}$(across the vertical dotted line in Fig. 1(b)). For comparison, the ideal field profile is again plotted using a black dotted line. The FEA results confirm that the computed magnetic field varies with Z in a manner consistent with a hyperbolic secant function and agrees well in magnitude with the ideal field throughout the operational Z-range of the magnetic plate.

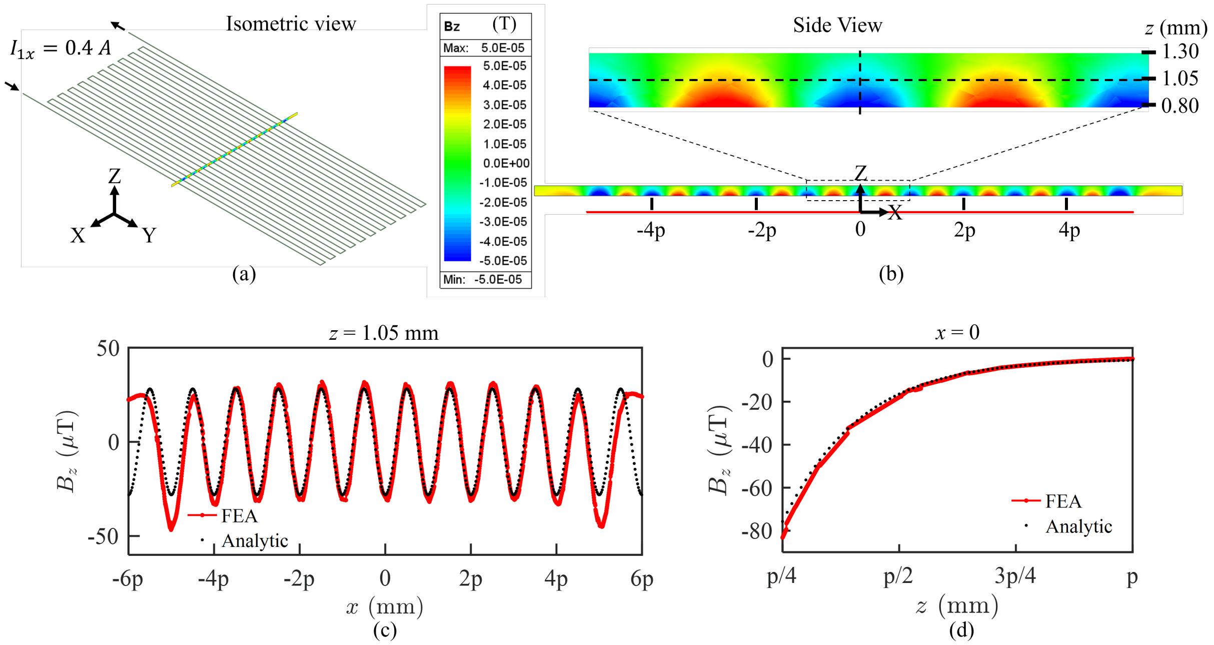


Figure 1: (a) Schematic showing isometric view of the track $I_{1x}$ used in the finite element analysis (FEA). The track consists of 22 parallel copper conductors, each with length 74 mm, width 127 $\mu$m, thickness 35 $\mu$m, and pitch $p = 2.54$ mm. (b) Simulated distribution of the vertical magnetic field component $B_z$ in the XZ-plane, from $x = -6p$ to $x = 6p$, and $z = 800\,\mu$m to $1300\,\mu$m. (c) Comparison of $B_z$ along the X-axis at $z = 1050\,\mu$m from FEA and analytical model. (d) Comparison of $B_z$ along the Z-axis at $x = 0\,\mu$m from FEA and analytical model. The close agreement between the FEA and analytical results validates the electromagnetic model described in the main manuscript.

# Supplementary Note 3: In-Plane Position Measurement System

The in-plane position of the magnetic plate in the acquired images is determined using a template-matching algorithm. A reference template $T(i,j)$, corresponding to the object to be tracked, is defined. The algorithm, given in Equation (8), computes the normalized cross-correlation function $C(x_i, y_i)$, and the coordinates $(x_i, y_i)$ at which $C(x_i, y_i)$ is maximized are identified as the in-plane position of the object. The resolution of this algorithm is limited to 1 pixel.

$$C(x,y) = \frac{\sum_{(i,j)} I(x+i, y+j)\,T(i,j)}{\sqrt{\sum_{(i,j)} [I(x+i,y+j)]^2} \cdot \sqrt{\sum_{(i,j)} [T(i,j)]^2}} \tag{8}$$

To improve resolution, sub-pixel accuracy of 0.01 pixels is achieved using a Newton–Raphson based refinement of the correlation peak [1, 3–5]. With a pixel size of 3.45 µm and an optical magnification of 20 (using the MC031MG-SY-UB camera from Ximea and the LMPLFLN20X objective lens from Olympus), the measurement resolution of the pixel-level

algorithm is 172 nm. Therefore, the sub-pixel algorithm achieves a theoretical resolution of approximately 1.72 nm.

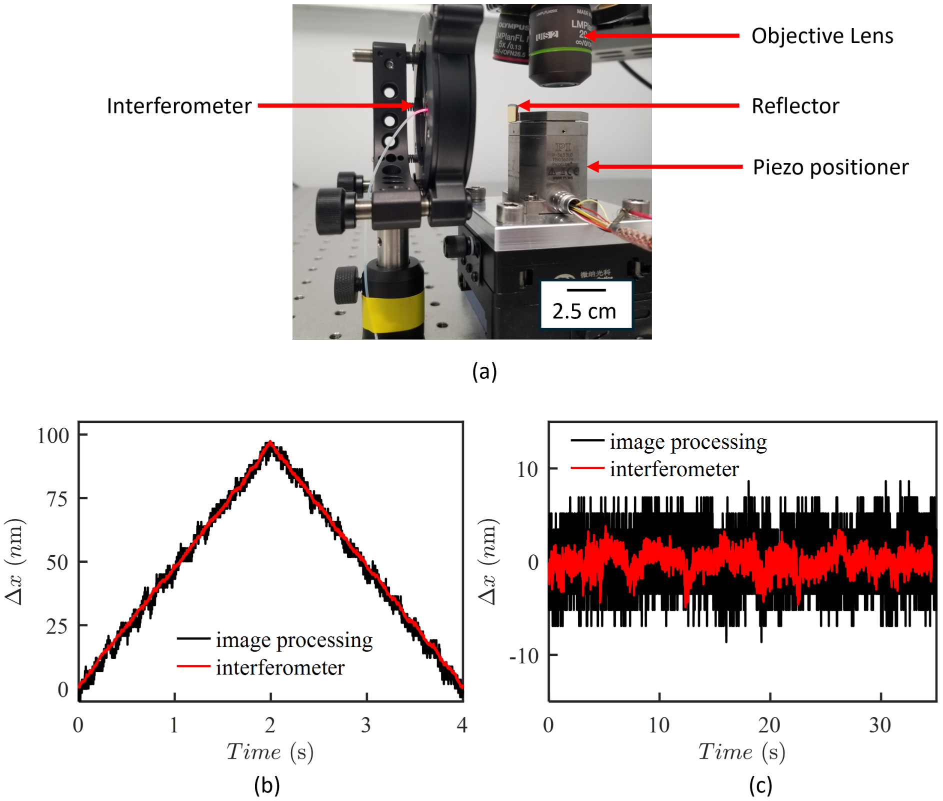


Figure 2: (a) Photograph of the experimental setup used to evaluate the in-plane position measurement system based on sub-pixel digital image cross-correlation. The X-displacement of the piezo positioner is simultaneously measured using the developed image-based system and an optical interferometer. A reflector is mounted on the piezo positioner to direct the laser beam toward the interferometer's sensor head. (b–c) Plots comparing the measured displacement from the image-based system and the interferometer. The results demonstrate that the developed system achieves nanometer-scale measurement accuracy.

The algorithm is implemented in MATLAB. Since the algorithm is computationally intensive, the time required for computing the position of a single acquired image comprising 2064 x 1544 pixels is relatively large, usually a few seconds. Therefore, first, we acquired a sequence of images of the moving magnetic plate at a high frame rate of approximately 1000 frames per second. Subsequently, we measured the position of the magnetic plate in the acquired images by processing the images using the developed algorithm.

To experimentally evaluate the positioning resolution of the developed system, we simultaneously tracked the X-motion of a piezo positioner (P-363 PicoCube$^{\mathrm{TM}}$, PI) using both the interferometer (PICOSCALE, SmarAct) and the image-based system. Figure 1(a) shows the experimental setup comprising the piezo-positioner, the interferometer, and the developed in-plane position measurement system based on sub-pixel digital image cross-correlation.

Figure 1(b) shows that the linear motion measured using both systems is nearly identical, validating the accuracy of the developed image-processing-based method. As shown in

Figure 1(c), the peak-to-peak measurement noise was 15 nm for the developed system and 8 nm for the interferometer. The root mean square (rms) positioning resolutions for the interferometer and the developed in-plane position measurement system were calculated to be 1 nm and 2.27 nm, respectively.

Finally, the motion range of the developed system is determined by the number of pixels in the camera sensor multiplied by the pixel size and divided by the magnification of the objective lens. For a 5X objective lens(LMPLFLN5X, Olympus), the resulting motion range is approximately 1.424 mm along the X-axis and 1.065 mm along the Y-axis.

# References


[1] K. Vikrant and G. Jayanth, "Diamagnetically levitated nanopositioners with large-range and multiple degrees of freedom," *Nature Communications*, vol. 13, no. 1, p. 3334, 2022.

[2] P. Romagnoli, R. Lecamwasam, S. Tian, J. Downes, and J. Twamley, "Controlling the motional quality factor of a diamagnetically levitated graphite plate," *Applied Physics Letters*, vol. 122, no. 9, 2023.

[3] P. Bing, X. Hui-Min, X. Bo-Qin, and D. Fu-Long, "Performance of sub-pixel registration algorithms in digital image correlation," *Measurement science and technology*, vol. 17, no. 6, p. 1615, 2006.

[4] X. Zhang, X. Zhang, H. Wu, J. Gan, and H. Li, "A high accuracy algorithm of displacement measurement for a micro-positioning stage," *Aip Advances*, vol. 7, no. 5, 2017.

[5] V. K. Singh, *Diamagnetically levitated nano positioners with large-range and multiple degrees of freedom.* PhD thesis, 2022.
